# Supplementary material for: SHED: A Newton-type algorithm for federated learning based on incremental Hessian eigenvector sharing
Source: arXiv:2202.05800 source file (2022-09-12)
Supplement: Supplementary file 1 [file Appendix_AColor.tex]

In this appendix, we include the complete proofs of the results of Section \ref{sec:generalConvex} for which only a proof sketch was provided.

\section*{Proof of Lemma~\ref{lemma:ArmijoLSs}}
The quadratic cost in $\boldsymbol{\theta}^t$ can be written as
		\begin{equation*}\label{eq:cost}
			f(\boldsymbol{\theta}^t) = f(\boldsymbol{\theta}^*) +  \bar{f}(\boldsymbol{\theta}^t).
		\end{equation*}
		with $\bar{f}(\boldsymbol{\theta}^t) = \frac{1}{2}(\boldsymbol{\theta}^t - \boldsymbol{\theta}^*)^T\mathbf{H}_{LS}(\boldsymbol{\theta}^t - \boldsymbol{\theta}^*)$. Given that $f(\boldsymbol{\theta}^*)$ does not depend on $\boldsymbol{\theta}^t$, we can focus on $\bar{f}(\boldsymbol{\theta}^t)$.\newline
		We have that
		\begin{equation}\label{eq:GetSuffCond}
			\begin{aligned}[b]
				\bar{f}(\boldsymbol{\theta}^t - \eta_t\mathbf{p}_t) &= \frac{1}{2}(\boldsymbol{\theta}^t -  \eta_t\mathbf{p}_t - \boldsymbol{\theta}^*)^T\mathbf{H}_{LS}(\boldsymbol{\theta}^t - \eta_t\mathbf{p}_t - \boldsymbol{\theta}^*)\\&
				\stackrel{(1)}{=} \bar{f}(\boldsymbol{\theta}^t) + \frac{1}{2} \eta_t^2\mathbf{p}_t^T \mathbf{H}_{LS}\mathbf{p}_t - \eta_t\mathbf{p}_t^T  \mathbf{g}_t\\&
				\stackrel{(2)}{=} \bar{f}(\boldsymbol{\theta}^t) - \eta_t\mathbf{p}_t^T(\hat{\mathbf{H}}_t - \eta_t\frac{\mathbf{H}_{LS}}{2})\mathbf{p}_t
			\end{aligned}
		\end{equation}
		where we have used identity $\mathbf{H}_{LS}(\boldsymbol{\theta}_t-\boldsymbol{\theta}^*) = \mathbf{g}_t$ and the fact that $ \mathbf{p}_t^T  \mathbf{g}_t =  \mathbf{p}_t^T\hat{\mathbf{H}}_t\hat{\mathbf{H}}_t^{-1}\mathbf{g}_t = \mathbf{p}_t^T\hat{\mathbf{H}}_t\mathbf{p}_t$ to get equality (1) and (2), respectively. We see that if 
		\begin{equation}\label{eq:SuffCondArmijo}
			\hat{\mathbf{H}}_t - \eta_t\mathbf{H}_{LS}/2 \geq \hat{\mathbf{H}}_t/2,    
		\end{equation}
		then Armijo-Goldstein condition (\ref{eq:Armijo}) is satisfied. Indeed, in that case,
		\begin{equation*}
			\begin{aligned}
				\bar{f}(\boldsymbol{\theta}^t) - \eta_t\mathbf{p}_t^T(\hat{\mathbf{H}}_t - \eta_t\frac{\mathbf{H}_{LS}}{2})\mathbf{p}_t &\leq \bar{f}(\boldsymbol{\theta}^t) - \frac{1}{2}\eta_t\mathbf{p}_t^T\hat{\mathbf{H}}_t\mathbf{p}_t\\& \leq \bar{f}(\boldsymbol{\theta}^t) - \alpha\eta_t\mathbf{p}_t^T\mathbf{g}_t.
			\end{aligned}
		\end{equation*}
		So, we need to find a sufficient condition on $\eta_t$ for (\ref{eq:SuffCondArmijo}) to be true. We see that (\ref{eq:SuffCondArmijo}) is equivalent to $\hat{\mathbf{H}}_t - \eta_t\mathbf{H}_{LS} \geq 0$. We have $\hat{\mathbf{H}}_t - \eta_t\mathbf{H}_{LS} = \frac{1}{M}\sum_{i = 1}^{M}\mathbf{V}^{(i)}(\hat{\boldsymbol{\Lambda}}_t^{(i)} - \eta_t\boldsymbol{\Lambda}_t^{(i)})\mathbf{V}^{(i)T}$, and, $\forall{i}$, all the elements of the diagonal matrix $\hat{\boldsymbol{\Lambda}}_t^{(i)} - \eta_t\boldsymbol{\Lambda}_t^{(i)}$ are positive if $\eta_t \leq \rho^{(i)}_t/\lambda_{q_t^{(i)}+1}^{(i)}$ (see Eq. (\ref{eq:theLambdas})), and we see that the choice (\ref{eq:conditionSS}) provides a sufficient condition to satisfy (\ref{eq:SuffCondArmijo}), from which we can conclude. 

\section*{Proof of Lemma \ref{Th:stepSizeConvex}}\label{proof:lemmaSS}
The following proof is similar to the proof for the beginning of the quadratically convergent phase in  centralized Newton method by \cite{ConvexOptimization}, page 490-491. We start with some definitions: given, at iteration $t$, $f({\x}^t)$ the cost, $\mathbf{g}_t = \nabla f({\x}^t)$ the gradient $\mathbf{H}_t = \nabla^2 f({\x}^t)$ the Hessian at ${\x}^t$, $\mathbf{H}_{k_t} = \nabla^2 f({\x}^{k_t})$ the Hessian at ${\x}^{k_t}$, and $\hat{\mathbf{H}}_t$ the global Hessian approximation of Algorithm~\ref{alg:2}, and with $\mathbf{p}_t = \hat{\mathbf{H}}_t^{-1}\mathbf{g}_t$. Define
\begin{equation}\label{eq:L9defs}
\begin{aligned}
    \bar{\sigma}_t^2 &:= \mathbf{p}_t^T\mathbf{g}_t =  \mathbf{g}_t^T\hat{\mathbf{H}}_t^{-1}\mathbf{g}_t,\\
    {\sigma}_t^2 &:= \mathbf{p}_t^T{\nabla^2f({\x}^t)}\mathbf{p}_t = \mathbf{p}_t^T{\mathbf{H}}_t\mathbf{p}_t,\\
    \Tilde{f}(\eta) &:= f({\x}^t - \eta\mathbf{p}_t), \ \ \Tilde{f}(0) = f({\x}^t),\\
    \Tilde{f}'(\eta) &:= \frac{\partial \Tilde{f}(\eta)}{\partial \eta} = -\nabla {f}({\x}^t - \eta\mathbf{p}_t)^T\mathbf{p}_t, \\
    \Tilde{f}''(\eta) &:= \frac{\partial^2 \Tilde{f}(\eta)}{\partial \eta^2} = \mathbf{p}_t^T\nabla^2 f({\x}^t - \eta \mathbf{p}_t)\mathbf{p}_t.
\end{aligned}
\end{equation}
Note that
\begin{equation}\label{eq:tildeInZero}
\begin{aligned}
    \Tilde{f}'(0) &= -\mathbf{g}_t^T\mathbf{p}_t = -\bar{\sigma}_t^2,\\
    \Tilde{f}''(0) &= \mathbf{p}_t^T\mathbf{H}_t\mathbf{p}_t = \sigma_t^2.
\end{aligned}
\end{equation}
 With the $\rho_m$ defined in the Lemma, it holds that $\hat{\mathbf{H}}_t \geq \rho_m, \ \ \forall{t}$. Thanks to the fact that the cost is $L$-Lipschitz (Assumption~\ref{ass:twice}), it holds that $\|\nabla^2f({\x}^t - \eta \mathbf{p}_t) - \nabla^2f({\x}^t)\| \leq \eta L\|\mathbf{p}_t\|$ and we have that
\begin{equation}\label{eq:Bound1L9}
    |\Tilde{f}''(\eta) - \Tilde{f}''(0)| = \mathbf{p}_t^T(\nabla^2f({\x}^t - \eta \mathbf{p}_t) - \nabla^2f({\x}^t))\mathbf{p}_t \leq \eta L\|\mathbf{p}_t\|^3\leq \eta L \frac{\bar{\sigma}^3({\x}^t)}{\rho_m^{3/2}}
\end{equation}
where the last inequality holds because $\rho_m\|\mathbf{p}_t\|^2 \leq \mathbf{p}_t^T\hat{\mathbf{H}}\mathbf{p}_t = \bar{\sigma}_t^2$. From (\ref{eq:Bound1L9}) it follows that 
\begin{equation}
    \Tilde{f}''(\eta) \leq \Tilde{f}''(0) + \eta L \frac{\bar{\sigma}^3({\x}^t)}{\rho_m^{3/2}} = \sigma_t^2 + \eta L \frac{\bar{\sigma}^3({\x}^t)}{\rho_m^{3/2}}.
\end{equation}
Similarly to \cite{ConvexOptimization}, page 490-491, we can now integrate both sides of the inequality getting 
\begin{equation*}
    \Tilde{f}'(\eta) \leq \Tilde{f}'(0)  + \eta\sigma_t^2 + \frac{\eta^2}{2}L\frac{\Bar{\sigma}_t^3}{\rho_m^{3/2}} = -\bar{\sigma}_t^2 + \eta\sigma_t^2 + \frac{\eta^2}{2}L\frac{\Bar{\sigma}_t^3}{\rho_m^{3/2}}.
\end{equation*}
By integrating again both sides of the inequality, we get, recalling that $\Tilde{f}(0) = f({\x}^t)$,
\begin{equation}\label{eq:Bound3L9}
\begin{aligned}
    \Tilde{f}(\eta) &= f({\x}^t - \eta\mathbf{p}_t) \leq f({\x}^t) -\eta\Bar{\sigma}_t^2 + \frac{\eta^2}{2}\sigma_t^2 + \frac{\eta^3}{6}L\frac{\Bar{\sigma}_t^3}{\rho_m^{3/2}}.
\end{aligned}
\end{equation}
Now, recalling $\mathbf{H}({\x}^{k_t}) \leq \hat{\mathbf{H}}_t$, we get that
\begin{equation}\label{eq:boundL9}
\begin{aligned}
    \sigma_t^2 = \mathbf{p}_t^T\mathbf{H}_t\mathbf{p}_t &= \mathbf{p}_t^T(\mathbf{H}_{k_t} + \mathbf{H}_t - \mathbf{H}_{k_t})\mathbf{p}_t =  \mathbf{p}_t^T\mathbf{H}_{k_t}\mathbf{p}_t + \mathbf{p}_t^T(\mathbf{H}_t - \mathbf{H}_{k_t})\mathbf{p}_t\\&\leq \mathbf{p}_t^T\hat{\mathbf{H}}_t\mathbf{p}_t + L\|\mathbf{p}_t\|^2\|{\x}^t - {\x}^{k_t}\| \leq \Bar{\sigma}_t^2 + \frac{L\Bar{\sigma}_t^2}{\rho_m}\|{\x}^t - {\x}^{k_t}\|,
\end{aligned}
\end{equation}
where we have used Lipschitz continuity, and the fact that $\mathbf{p}_t^T\hat{\mathbf{H}}_t\mathbf{p}_t = \Bar{\sigma}_t^2$ and $\rho_m\|\mathbf{p}_t\|^2 \leq {\Bar{\sigma}_t^2}$. \newline
Next, setting $\eta = 1$ and plugging (\ref{eq:boundL9}) in (\ref{eq:Bound3L9}), we get 
\begin{equation}\label{eq:IneqArmijo}
\begin{aligned}
    f({\x}^t - \mathbf{p}_t) \leq f({\x}^t) -\Bar{\sigma}_t^2 + \frac{\sigma_t^2}{2} + \frac{L}{6}\frac{\Bar{\sigma}_t^3}{\rho_m^{3/2}}
    &\leq f({\x}^t) - \frac{\Bar{\sigma}_t^2}{2} + \frac{L\Bar{\sigma}_t^2}{2\rho_m}\|{\x}^t - {\x}^{k_t}\| + \frac{L}{6}\frac{\Bar{\sigma}_t^3}{\rho_m^{3/2}}
    \\&\leq f({\x}^t) - {\Bar{\sigma}_t^2}(\frac{1}{2} - \frac{L}{2\rho_m}\|{\x}^t - {\x}^{k_t}\| - \frac{L}{6}\frac{\Bar{\sigma}_t}{\rho_m^{3/2}})\\&=
    f({\x}^t) - \mathbf{p}_t^T\mathbf{g}_t(\frac{1}{2} - \frac{L}{2\rho_m}\|{\x}^t - {\x}^{k_t}\| - \frac{L}{6}\frac{\Bar{\sigma}_t}{\rho_m^{3/2}}).
\end{aligned}
\end{equation}
In order for (\ref{eq:IneqArmijo}) to satisfy the Armijo-Goldstein condition (\ref{eq:Armijo}) for any parameter $\alpha \in (0, 1/2)$ we see that
\begin{equation}
    \frac{1}{2} - \frac{L}{2\rho_m}\|{\x}^t - {\x}^{k_t}\| - \frac{L}{6}\frac{\Bar{\sigma}_t}{\rho_m^{3/2}} \geq \alpha
\end{equation}
provides a sufficient condition. The above inequality can be written as
\begin{equation}
    3\rho_m\|{\x}^t - {\x}^{k_t}\| + \rho_m^{1/2}{\bar{\sigma}_t} \leq \frac{3\rho_m^2}{L}(1 - 2\alpha).
\end{equation}
We have that $\bar{\sigma}_t^2 = \mathbf{g}_t^T\hat{\mathbf{H}}^{-1}\mathbf{g}_t \leq \|\mathbf{g}_t\|^2/\rho_m$, which implies $\rho_m^{1/2}\|\sigma_t\| \leq \|\mathbf{g}_t\|$. Furthermore, by triangular inequality, we have $\|{\x}^t - {\x}^{k_t}\| \leq \|{\x}^t - {\x}^*\| + \|{\x}^{k_t} - {\x}^*\|$. Therefore, we see that if 
\begin{equation}
    3\rho_m(\|{\x}^t - {\x}^*\| + \|{\x}^{k_t} - {\x}^*\|) + \|\mathbf{g}_t\|^{\red{\cancel{2}}} \leq \frac{3\rho_m^2}{L}(1 - 2\alpha),
\end{equation}
then the Armijo-Goldstein condition is satisfied and $\eta = 1$ is chosen by the backtracking algorithm, proving the Lemma.

\section*{Proof of Theorem \ref{Th:expConvergence}}
1) We suppose to be in the condition in which $t$ is such that, for some $\bar{t}$, $t \geq \bar{t}$ implies that $\eta_t = 1$ is chosen by Armijo backtracking line search. From Lemma~\ref{Th:stepSizeConvex} and Corollary~\ref{Cor:ThereExists}, such $\bar{t}$ exists. From (\ref{eq:convBound}) of Theorem \ref{Th:theorem_2}, we have that, for $t \geq \bar{t}$
\begin{equation}\label{eq:linConv}
\begin{aligned}
    \|\boldsymbol{\theta}^{t+1} - \boldsymbol{\theta}^*\| \leq \bar{c}_t\|\boldsymbol{\theta}^t - \boldsymbol{\theta}^*\|
\end{aligned}
\end{equation}
where 
\begin{equation}\label{eq:barc}
\begin{aligned}
    \bar{c}_t &= 1-\frac{\bar{\lambda}_{n,t}}{\bar{\rho}_t} + \frac{L}{\bar{\rho}_t}\|\boldsymbol{\theta}^{k_t} - \boldsymbol{\theta}^t\| + \frac{L}{2\bar{\rho}_t}\|\boldsymbol{\theta}^t - \boldsymbol{\theta}^*\| \\& \leq  1-\frac{\bar{\lambda}_{n,t}}{\bar{\rho}_t} + \frac{L}{\bar{\rho}_t}\|\boldsymbol{\theta}^{k_t} - \boldsymbol{\theta}^*\| + B'\|\boldsymbol{\theta}^t - \boldsymbol{\theta}^*\|,
\end{aligned}
\end{equation}
where $B' = \frac{L}{\bar{\rho}_t} + \frac{L}{2\bar{\rho}_t}$, and where we have used triangular inequality to get $\|\boldsymbol{\theta}^{k_t} - \boldsymbol{\theta}^t\| \leq \|\boldsymbol{\theta}^{k_t} - \boldsymbol{\theta}^*\| + \|\boldsymbol{\theta}^{t} - \boldsymbol{\theta}^*\|$.  Given Assumption \ref{th:AssDelayBound} and Corollary \ref{corollary:convergence}, we see that there surely exists $t'$ such that for all $t \geq t'$, $\bar{c}_t < 1$, because $k_t = t-\tau$, with $\tau$ bounded, and this proves (\ref{eq:linConvergence}).\\
2) From (\ref{eq:linConvergence}), letting $a_* \in (0, 1)$ be the Lyapunov exponent of $\|\x^t - \x^*\|$, we get, considering $\bar{c}_t$ and $B'$ as in (\ref{eq:barc}), 
\begin{equation*}
    \begin{aligned}
        \bar{c}_t &\leq 1-\frac{\bar{\lambda}_{n,t}}{\bar{\rho}_t} + \frac{L}{\bar{\rho}_t}\|\boldsymbol{\theta}^{k_t} - \boldsymbol{\theta}^*\| + B'\|\boldsymbol{\theta}^t - \boldsymbol{\theta}^*\|\\&\leq
        1-\frac{\bar{\lambda}_{n,t}}{\bar{\rho}_t} + \frac{L}{\bar{\rho}_t}C_1{a_*}^{t-T} + B'C_2{a_*}^{t}\\&=
        1-\frac{\bar{\lambda}_{n,t}}{\bar{\rho}_t} + Ba_*^{t},
    \end{aligned}
\end{equation*}
where $B = \frac{L}{\bar{\rho}_t}C_1a_*^{-T} + B'C_2$, bounded. For any iteration $t$, we can write $\|\x^{t+1} - \x^*\| \leq \bar{c}_t\|\x^t - \x^*\|$ for some $\bar{c}_t$ that could also be greater than one, if $t < t'$, but it is easy to see that $\bar{c}_t$ is always bounded. Now, we consider $\bar{a} := \limsup_{t}{(\prod_{k = 1}^{t}{\bar{c}_k})^{1/t}}$. It is straightforward to see that, as in the least squares case, it is $\bar{a} \geq a_*$. We can write
\begin{equation*}
\begin{aligned}
    \log{\bar{a}} = \limsup_{t}{\frac{1}{t}}\sum_{k = 1}^{t}\log{\bar{c}_k} &= \limsup_{t}{\frac{1}{t}}(\sum_{k = 1}^{\bar{t}}\log{\bar{c}_k} + \sum_{k = \bar{t} + 1}^{t}\log{\bar{c}_k})\\& = \limsup_{t}{\frac{1}{t}}(\sum_{k = \bar{t} + 1}^{t}\log{\bar{c}_k})
\end{aligned}
\end{equation*}
where the last equality follows from the boundedness of $\bar{c}_k$. We get
\begin{equation*}
\begin{aligned}
    \log{\bar{a}} = \limsup_{t}{\frac{1}{t}}(\sum_{k = \bar{t} + 1}^{t}\log{\bar{c}_k}) &\leq \limsup_{t}\frac{1}{t}\sum_{k = \bar{t} +1}^{t}\log{(1-\frac{\bar{\lambda}_{n,k}}{\bar{\rho}_k} + B{a_*}^k)}\\&= \limsup_{t}\frac{1}{t}\sum_{k = \bar{t} +1}^{t}\log{(1-\frac{\bar{\lambda}_{n,k}}{\bar{\rho}_k})} + \log{(1 + \frac{B{a_*}^{k}}{1 - \frac{\bar{\lambda}_{n,k}}{\bar{\rho}_k}})}.
\end{aligned}
\end{equation*}
We see that the last term is 
\begin{equation*}
    \log{(1 + \frac{B{a_*}^k}{1 - \frac{\bar{\lambda}_{n,k}}{\bar{\rho}_k}})} \leq \frac{B{a_*}^k}{1 - \frac{\bar{\lambda}_{n,k}}{\bar{\rho}_k}}\leq {\bar{B}{a_*}^k}
\end{equation*}
that comes from the identity $\log{(1+x)} \leq x$, and where $\bar{B} = \max_{k}\frac{1}{{1 - \frac{\bar{\lambda}_{n,k}}{\bar{\rho}_k}}}$, bounded because we assumed $q_t^{(i)} < n-1, \forall{i}, \forall{t}$ and thus $\bar{\rho}_k > \bar{\lambda}_{n,k}$ (note that we can assume, without loss of generality, that all eigenvalues are different). Now, we see that 
\begin{equation*}
    \limsup_{t}{\frac{1}{t}}\sum_{k = 1}^{t}{\bar{B}{a_*}^k} = \limsup_{t}\frac{1}{t}{\bar{B}}(\frac{1 - {a_*}^{t+1}}{1 - a_*} - 1) = 0.
\end{equation*}
Hence, we get 
\begin{equation}\label{eq:logIdentity}
    \log{\bar{a}} = \limsup_{t}\frac{1}{t}\sum_{k = 1}^{t}\log{(1-\frac{\bar{\lambda}_{n,k}}{\bar{\rho}_k})}.
\end{equation}
Now we use local Lipschitz continuity (Assumption \ref{ass:localLCont}) to conclude the proof. It is straightforward to see that Lipschitz continuity of $f^{(i)}(\boldsymbol{\theta})$ implies that, for any $k \in \{1,..., n\}$, $|\lambda_k^{(i)}(\x) - \lambda_k^{(i)}(\x^*)| \leq \bar{L}\|\x - \x^*\|$, which in turn implies $\lambda_k^{(i)}(\x) \geq \lambda_k^{(i)}(\x^*) - \bar{L}\|\x - \x^*\|$ and $\lambda_k^{(i)}(\x) \leq \lambda_k^{(i)}(\x^*) + \bar{L}\|\x - \x^*\|$. It follows that 
\begin{equation*}
    \begin{aligned}
        \log{\bar{a}} &\leq \limsup_{t}\frac{1}{t}\sum_{k = 1}^{t}\log{(1 - \frac{\bar{\lambda}_n^{o} - \bar{L}\|\x^{k_t} - \x^*\|}{\bar{\rho}_k^{o} + \bar{L}\|\x^{k_t} - \x^*\|})}\\&\stackrel{(1)}{=} \limsup_{t}\frac{1}{t}\sum_{k = 1}^{t}\log{(1 - \frac{\bar{\lambda}_n^{o} }{\bar{\rho}_k^{o} + \bar{L}\|\x^{k_t} - \x^*\|})}\\& = \limsup_{t}\frac{1}{t}\sum_{k = 1}^{t}\log{(\frac{\bar{\rho}_k^{o} - \bar{\lambda}_n^{o} + \bar{L}\|\x^{k_t} - \x^*\|}{\bar{\rho}_k^{o} + \bar{L}\|\x^{k_t} - \x^*\|})}\\&\leq  \limsup_{t}\frac{1}{t}\sum_{k = 1}^{t}\log{(1 - \frac{ \bar{\lambda}_n^{o}}{{\bar{\rho}_k^{o}}} + \frac{\bar{L}\|\x^{k_t} - \x^*\|}{\bar{\rho}_k^{o}})}\\&\stackrel{(2)}{=} \limsup_{t}\frac{1}{t}\sum_{k = 1}^{t}\log{(1 - \frac{ \bar{\lambda}_n^{o}}{{\bar{\rho}_k^{o}}})}
    \end{aligned}
\end{equation*}
where equalities (1) and (2) follow from calculations equivalent to the ones used to obtain (\ref{eq:logIdentity}).\\ 3) Starting from 2), we can apply calculations analogous to the ones used in equation (\ref{eq:periodicObtain}) of Lemma \ref{lemma:LyapLSs}.

\section*{Proof of Theorem \ref{th:suplin}}
We show that the Lyapunov exponent is $a_* = 0$. From Lemma~\ref{Th:stepSizeConvex} and Corollary~\ref{Cor:ThereExists}, there exists a $\bar{t}$ such that $\eta_t = 1$ is chosen by the backtracking line search for any $t \geq \bar{t}$. Local linear convergence proven in Theorem \ref{Th:expConvergence} implies that there exists a $t'$ such that, for all $t \geq t'$, $ \|\boldsymbol{\theta}^{t+1} - \boldsymbol{\theta}^*\| \leq \bar{c}_t\|\boldsymbol{\theta}^t - \boldsymbol{\theta}^*\|$, with $\bar{c}_t < 1$. In particular, we have, from (\ref{eq:barc})
\begin{equation*}\label{eq:cbarAgain}
\bar{c}_t \leq 1-\frac{\bar{\lambda}_{n,t}}{\bar{\rho}_t} + \frac{L}{\bar{\rho}_t}\|\boldsymbol{\theta}^{k_t} - \boldsymbol{\theta}^*\| + \frac{3L}{2\bar{\rho}_t}\|\boldsymbol{\theta}^t - \boldsymbol{\theta}^*\|.    
\end{equation*}
Linear convergence implies that, for some constant $C > 0$, we can write $\|\boldsymbol{\theta}^{t} - \boldsymbol{\theta}^*\| \leq Ca^{t}$ for some $a \in (0,1)$. Furthermore, given that $k_t = t - \tau$ with $\tau$ bounded, we have $\|\x^{k_t} - \x^*\| = \|\x^{t-\tau} - \x^*\| \leq C'a^{t}$ for some bounded $C'$. 

It is easy to see that, given that the algorithm convergence is at least linear with some Lyapunov exponent $a_*$, $\bar{a}$ defined as  $\bar{a} := \limsup_{t}{(\prod_{k = 1}^{t}{\bar{c}_k})^{1/t}}$ is such that $\bar{a} \geq a_*$. For $k < t'$, $\bar{c}_k$ is some bounded value that could be greater than $1$. 

To prove the Theorem we use the fact that, for $q_t^{(i)} = n'$, $\hat{\rho}_t^{(i)} = \hat{\lambda}_{n, t}^{(i)}$ for all $i$. Let $t = Rn' + T'$ for some $T' < n'$ and $R \in \mathbb{N}$. Given the conditions required by the Theorem, we see that $q_{kn'}^{(i)} = n'$ for $k = 1,2,...,R$. When $t = kn' \geq \bar{t}$, $\bar{c}_t$ is as in (\ref{eq:cbarAgain}), and we have $q_t^{(i)} = n'$ and $\hat{\rho}_{kn'}^{(i)} = \hat{\lambda}_{n, kn'}^{(i)}$, so $\bar{\rho}_{kn'} = \bar{\lambda}_{n,kn'}$. Consequently, $1-\frac{\bar{\lambda}_{n, kn'}}{\bar{\rho}_{kn'}} = 0$ and
\begin{equation*}
\bar{c}_{kn'} = \frac{L}{\bar{\rho}_{kn'}}\|\boldsymbol{\theta}^{kn' - n'} - \boldsymbol{\theta}^*\| + \frac{3L}{2\bar{\rho}_{kn'}}\|\boldsymbol{\theta}^{kn'} - \boldsymbol{\theta}^*\| \leq Ba^{kn'}    
\end{equation*}
for some bounded $B$.
Taking the logarithm of $\bar{a}$, we can then write, letting $l$ be the positive integers such that $l \geq k'$, with $k'$ a sufficiently big integer in order to have $k'n' \geq \bar{t}$
\begin{equation*}
\begin{aligned}
    \log{\bar{a}} &= \limsup_{t}{\log{(\prod_{k = 1}^{t}{\bar{c}_k})^{1/t}}} = \limsup_{t}{\frac{1}{t}}\sum_{k = 1}^{t}\log{\bar{c}_k}\\
    &= \limsup_{R}\frac{1}{Rn' + T'}(\sum_{\substack{k = 1\\ k \neq ln'}}^{Rn' + T'}{\log{\bar{c}_k}} + \sum_{k = k'}^{R}{\log{Ba^{kn'}}}),
\end{aligned}
\end{equation*}
The first term between parentheses is bounded in the following way: $\sum_{\substack{k = 1\\ k \neq ln'}}^{Rn' + T'}{\log{\bar{c}_k}} \leq C(Rn' + T')$, for some constant $C$. The second term between parentheses can be written as 
\begin{equation*}
\begin{aligned}
    \sum_{k = k'}^{R}\log{Ba^{kn'}} &= (R-k'+1)\log{B} + \sum_{k = 1}^{R}\log{a^{kn'}} - \sum_{k = 1}^{k'}\log{a^{kn'}}\\&\leq R\log{B} + (\frac{n'R^2}{2}- {n'{(k'+1)}^2})\log{a}.
\end{aligned}
\end{equation*}
The previous expression thus becomes:
\begin{equation*}
\begin{aligned}
    \log{\bar{a}} &\leq \limsup_{R}C + \frac{R\log{B} + ({n'R^2}{/2}- {n'{(k'+1)}^2})\log{a}}{Rn' + T'}\\& = C + \frac{\log{B}}{n'} + \limsup_{R}\frac{R}{2}\log{a} = -\infty
\end{aligned}
\end{equation*}
so $0 \leq a_* \leq \bar{a} = 0 \implies a_* = 0$.

\newpage
