# Supplementary material for: SHED: A Newton-type algorithm for federated learning based on incremental Hessian eigenvector sharing
Source: arXiv:2202.05800 source file (2022-09-12)
Supplement: Supplementary file 5 [file Appendix_A_old.tex]

In this appendix, we include the complete proofs of the results of Section \ref{sec:generalConvex} for which only a proof sketch was provided.

\section*{Proof of Lemma \ref{Th:stepSizeConvex}}\label{proof:lemmaSS}
To prove this lemma, we use Taylor expansion of the cost and use the result of Lemma \ref{lemma:ArmijoLSs} ensuring that $\eta_t = \min_{i = 1, ..., M}{{\rho_t^{(i)}}/{\lambda_{q^{(i)}_t+1}^{(i)}}}$ is accepted in the linear regression case. The Taylor expansion of the cost in $\boldsymbol{\theta}^t$ around $\x^*$ is 
\begin{equation}\label{eq:CostExpansion}
    f(\boldsymbol{\theta}^t) = f(\boldsymbol{\theta}^*) + \frac{1}{2}(\boldsymbol{\theta}^t - \boldsymbol{\theta}^*)^T\mathbf{H}^*(\boldsymbol{\theta}^t - \boldsymbol{\theta}^*) + k_0( {\x}^t )
\end{equation}
where $k_0( {\x}^t )$ is such that
\begin{equation*}
    \lim_{\x^t \rightarrow \x^*}\frac{k_0({\x}^t)}{\|\boldsymbol{\theta}^t - \boldsymbol{\theta}^*\|^2} = 0
\end{equation*}
Similarly, in $\boldsymbol{\theta}^{t+1}$, the expansion is
\begin{equation*}
\begin{aligned}
    f(\boldsymbol{\theta}^{t+1}) = f(\boldsymbol{\theta}^*) + \frac{1}{2}(\boldsymbol{\theta}^t - \boldsymbol{\theta}^* - \eta_t\mathbf{p}_t)^T\mathbf{H}^*(\boldsymbol{\theta}^t &- \boldsymbol{\theta}^* - \eta_t\mathbf{p}_t)\\& + k_1({\x}^t)
\end{aligned}
\end{equation*}
where $\mathbf{p}_t = \hat{\mathbf{H}}_t^{-1}\mathbf{g}_t$, and $k_1({\x}^t)$ is such that 
\begin{equation*}
    \lim_{\x^t \rightarrow \x^*}\frac{k_1({\x}^t)}{\|\boldsymbol{\theta}^t - \boldsymbol{\theta}^*\|^2} = 0.
\end{equation*}
We can rewrite $f(\boldsymbol{\theta}^{t+1})$ as
\begin{equation*}
\begin{aligned}
    f(\boldsymbol{\theta}^{t+1}) = & f(\boldsymbol{\theta}^*) + \frac{1}{2}(\boldsymbol{\theta}^t - \boldsymbol{\theta}^*)^T\mathbf{H}^*(\boldsymbol{\theta}^t - \boldsymbol{\theta}^*)\\& 
    + \frac{1}{2}\eta_t^2\mathbf{p}_t^T\mathbf{H}^*\mathbf{p}_t - \eta_t\mathbf{p}_t^T\mathbf{H}^*({\x}^t - {\x}^*) + k_1({\x}^t),
\end{aligned}
\end{equation*}
the gradient can be expanded as $\mathbf{g}_t = \mathbf{H}^*(\boldsymbol{\theta}^t - \boldsymbol{\theta}^*) + \boldsymbol{\nu}_0({\x}^t)$ where $\boldsymbol{\nu}_0({\x}^t)$ is such that . 
\begin{equation*}
    \lim_{\x^t \rightarrow \x^*}\frac{\|\boldsymbol{\nu}_0({\x}^t)\|}{\|\boldsymbol{\theta}^t - \boldsymbol{\theta}^*\|} = 0
\end{equation*}
Consequently, defining $k_2({\x}^t) := \eta_t\mathbf{p}_t^T\boldsymbol{\nu}_0({\x}^t)$, we see that it is such that 
\begin{equation*}
    \lim_{\x^t \rightarrow \x^*}\frac{k_2({\x}^t)}{\|\boldsymbol{\theta}^t - \boldsymbol{\theta}^*\|^2} = 0,
\end{equation*}
and defining $k({\x}^t) := -k_0({\x}^t) + k_1({\x}^t) + k_2({\x}^t)$, using identity $\mathbf{p}_t^T\mathbf{g}_t = \mathbf{p}_t^T\hat{\mathbf{H}}_t\mathbf{p}_t$ and Eqn. (\ref{eq:CostExpansion}), we can write
\begin{equation*}
    f(\boldsymbol{\theta}^{t+1}) = f(\boldsymbol{\theta}^{t}) - \eta_t\mathbf{p}_t^T(\hat{\mathbf{H}}_t-\eta_t\frac{\mathbf{H}}{2}^*)\mathbf{p}_t + k({\x}^t).
\end{equation*}
 $\hat{\mathbf{H}}_t$ can be written as $\hat{\mathbf{H}}_t = \hat{\mathbf{H}}^*_t + \mathbf{N}_0({\x^{k_t}})$, with 
 \begin{equation*}
    \lim_{\x^{k_t} \rightarrow \x^*}\|\mathbf{N}_0({{\x}^{k_t}})\| = 0,
\end{equation*}
  while $\hat{\mathbf{H}}^*_t$ is defined as in (\ref{eq:aggregation}) but with $\x^{k_t^{(i)}} = \x^*, \ \forall{i}$. Defining $\bar{k}({\x^{k_t}}) := \eta_t\mathbf{p}_t^T\mathbf{N}_0({\x^{k_t}})\mathbf{p}_t$, we have 
\begin{equation*}
    \lim_{\x^{k_t} \rightarrow \x^*}\frac{\bar{k}({\x^{k_t}})}{\|\boldsymbol{\theta}^t - \boldsymbol{\theta}^*\|^2} = 0,
\end{equation*}
 We can then write
\begin{equation*}
    f(\boldsymbol{\theta}^{t+1}) = f(\boldsymbol{\theta}^{t}) - \eta_t\mathbf{p}_t^T(\hat{\mathbf{H}}_t^*-\eta_t\frac{\mathbf{H}}{2}^*)\mathbf{p}_t - \bar{k}({{\x}^{k_t}}) + k({{\x}^{t}}).
\end{equation*}
From Corollary \ref{corollary:ArmijoLSs}, we know that for the choice of $\rho_t^{(i)} = \rho_t^{(i)*}$ we have that $\bar{\eta}_t = 1$ is such that
\begin{equation*}
    \hat{\mathbf{H}}_t^*-\bar{\eta}_t\frac{\mathbf{H}}{2}^* \geq \frac{\hat{\mathbf{H}}_t^*}{2} = \frac{\hat{\mathbf{H}}_t}{2} - \frac{\mathbf{N}_0({\x}^{k_t})}{2},
\end{equation*}
and thus we can write
\begin{equation*}
\begin{aligned}
     f(\boldsymbol{\theta}^{t+1}) &\leq f(\boldsymbol{\theta}^{t}) - \frac{1}{2}\bar{\eta}_t\mathbf{p}_t^T\mathbf{g}_t - \frac{\bar{k}({\x}^{k_t})}{2} + k({\x}^{t})\\&
     \leq f(\boldsymbol{\theta}^{t}) - \alpha\bar{\eta}_t\mathbf{p}_t^T\mathbf{g}_t - \delta\bar{\eta}_t\mathbf{p}_t^T\mathbf{g}_t - \frac{\bar{k}({\x}^{k_t})}{2} + k({\x}^{t})
\end{aligned}
\end{equation*}
where we have written $1/2 = \alpha - \delta$, for some $\alpha, \delta \in (0, 1/2)$, with $\delta = 1/2 - \alpha$. Given that $\bar{\eta}_t\mathbf{p}_t^T\mathbf{g}_t >0$ and that 
\begin{equation*}
    \lim_{\x^{k_t} \rightarrow \x^*}\frac{{\bar{k}({\x}^{k_t})}/{2} + k({\x}^{t})}{\delta\bar{\eta}_t\mathbf{p}_t^T\mathbf{g}_t} = 0,
\end{equation*}
because $\mathbf{p}_t^T\mathbf{g}_t \propto \|\x^t - \x^*\|^2$. We see that, thanks to the fact that $k_t = t -\tau$ with $\tau$ bounded, there exists some $\bar{t}$ such that for any $t \geq \bar{t}$, $|\frac{\bar{k}({\x}^{k_t})}{2}+k({\x}^{t})| \leq \delta\bar{\eta}_t\mathbf{p}_t^T\mathbf{g}_t$, and so $\bar{\eta}_t = 1$ is chosen for any $t \geq \bar{t}$.
\section*{Proof of Theorem \ref{Th:expConvergence}}
1) We suppose to be in the condition in which $t$ is such that, for some $\bar{t}$, $t \geq \bar{t}$ implies that $\eta_t = 1$ is chosen by Armijo backtracking line search. From Lemma \ref{Th:stepSizeConvex}, such $\bar{t}$ exists. From (\ref{eq:convBound}) of Theorem \ref{Th:theorem_2}, we have that, for $t \geq \bar{t}$
\begin{equation}\label{eq:linConv}
\begin{aligned}
    \|\boldsymbol{\theta}^{t+1} - \boldsymbol{\theta}^*\| \leq \bar{c}_t\|\boldsymbol{\theta}^t - \boldsymbol{\theta}^*\|
\end{aligned}
\end{equation}
where 
\begin{equation}\label{eq:barc}
\begin{aligned}
    \bar{c}_t &= 1-\frac{\bar{\lambda}_{n,t}}{\bar{\rho}_t} + \frac{L}{\bar{\rho}_t}\|\boldsymbol{\theta}^{k_t} - \boldsymbol{\theta}^t\| + \frac{L}{2\bar{\rho}_t}\|\boldsymbol{\theta}^t - \boldsymbol{\theta}^*\| \\& \leq  1-\frac{\bar{\lambda}_{n,t}}{\bar{\rho}_t} + \frac{L}{\bar{\rho}_t}\|\boldsymbol{\theta}^{k_t} - \boldsymbol{\theta}^*\| + B'\|\boldsymbol{\theta}^t - \boldsymbol{\theta}^*\|,
\end{aligned}
\end{equation}
where $B' = \frac{L}{\bar{\rho}_t} + \frac{L}{2\bar{\rho}_t}$, and where we have used triangular inequality to get $\|\boldsymbol{\theta}^{k_t} - \boldsymbol{\theta}^t\| \leq \|\boldsymbol{\theta}^{k_t} - \boldsymbol{\theta}^*\| + \|\boldsymbol{\theta}^{t} - \boldsymbol{\theta}^*\|$.  Given Assumption \ref{th:AssDelayBound} and Corollary \ref{corollary:convergence}, we see that there surely exists $t'$ such that for all $t \geq t'$, $\bar{c}_t < 1$, because $k_t = t-\tau$, with $\tau$ bounded, and this proves (\ref{eq:linConvergence}).\\
2) From (\ref{eq:linConvergence}), letting $a_* \in (0, 1)$ be the Lyapunov exponent of $\|\x^t - \x^*\|$, we get, considering $\bar{c}_t$ and $B'$ as in (\ref{eq:barc}), 
\begin{equation*}
    \begin{aligned}
        \bar{c}_t &\leq 1-\frac{\bar{\lambda}_{n,t}}{\bar{\rho}_t} + \frac{L}{\bar{\rho}_t}\|\boldsymbol{\theta}^{k_t} - \boldsymbol{\theta}^*\| + B'\|\boldsymbol{\theta}^t - \boldsymbol{\theta}^*\|\\&\leq
        1-\frac{\bar{\lambda}_{n,t}}{\bar{\rho}_t} + \frac{L}{\bar{\rho}_t}C_1{a_*}^{t-T} + B'C_2{a_*}^{t}\\&=
        1-\frac{\bar{\lambda}_{n,t}}{\bar{\rho}_t} + Ba_*^{t},
    \end{aligned}
\end{equation*}
where $B = \frac{L}{\bar{\rho}_t}C_1a_*^{-T} + B'C_2$, bounded. For any iteration $t$, we can write $\|\x^{t+1} - \x^*\| \leq \bar{c}_t\|\x^t - \x^*\|$ for some $\bar{c}_t$ that could also be greater than one, if $t < t'$, but it is easy to see that $\bar{c}_t$ is always bounded. Now, we consider $\bar{a} := \limsup_{t}{(\prod_{k = 1}^{t}{\bar{c}_k})^{1/t}}$. It is straightforward to see that, as in the least squares case, it is $\bar{a} \geq a_*$. We can write
\begin{equation*}
\begin{aligned}
    \log{\bar{a}} = \limsup_{t}{\frac{1}{t}}\sum_{k = 1}^{t}\log{\bar{c}_k} &= \limsup_{t}{\frac{1}{t}}(\sum_{k = 1}^{\bar{t}}\log{\bar{c}_k} + \sum_{k = \bar{t} + 1}^{t}\log{\bar{c}_k})\\& = \limsup_{t}{\frac{1}{t}}(\sum_{k = \bar{t} + 1}^{t}\log{\bar{c}_k})
\end{aligned}
\end{equation*}
where the last equality follows from the boundedness of $\bar{c}_k$. We get
\begin{equation*}
\begin{aligned}
    \log{\bar{a}} = \limsup_{t}{\frac{1}{t}}(\sum_{k = \bar{t} + 1}^{t}\log{\bar{c}_k}) &\leq \limsup_{t}\frac{1}{t}\sum_{k = \bar{t} +1}^{t}\log{(1-\frac{\bar{\lambda}_{n,k}}{\bar{\rho}_k} + B{a_*}^k)}\\&= \limsup_{t}\frac{1}{t}\sum_{k = \bar{t} +1}^{t}\log{(1-\frac{\bar{\lambda}_{n,k}}{\bar{\rho}_k})} + \log{(1 + \frac{B{a_*}^{k}}{1 - \frac{\bar{\lambda}_{n,k}}{\bar{\rho}_k}})}.
\end{aligned}
\end{equation*}
We see that the last term is 
\begin{equation*}
    \log{(1 + \frac{B{a_*}^k}{1 - \frac{\bar{\lambda}_{n,k}}{\bar{\rho}_k}})} \leq \frac{B{a_*}^k}{1 - \frac{\bar{\lambda}_{n,k}}{\bar{\rho}_k}}\leq {\bar{B}{a_*}^k}
\end{equation*}
that comes from the identity $\log{(1+x)} \leq x$, and where $\bar{B} = \max_{k}\frac{1}{{1 - \frac{\bar{\lambda}_{n,k}}{\bar{\rho}_k}}}$, bounded because we assumed $q_t^{(i)} < n-1, \forall{i}, \forall{t}$ and thus $\bar{\rho}_k > \bar{\lambda}_{n,k}$ (note that we can assume, without loss of generality, that all eigenvalues are different). Now, we see that 
\begin{equation*}
    \limsup_{t}{\frac{1}{t}}\sum_{k = 1}^{t}{\bar{B}{a_*}^k} = \limsup_{t}\frac{1}{t}{\bar{B}}(\frac{1 - {a_*}^{t+1}}{1 - a_*} - 1) = 0.
\end{equation*}
Hence, we get 
\begin{equation}\label{eq:logIdentity}
    \log{\bar{a}} = \limsup_{t}\frac{1}{t}\sum_{k = 1}^{t}\log{(1-\frac{\bar{\lambda}_{n,k}}{\bar{\rho}_k})}.
\end{equation}
Now we use local Lipschitz continuity (Assumption \ref{ass:localLCont}) to conclude the proof. It is straightforward to see that Lipschitz continuity of $f^{(i)}(\boldsymbol{\theta})$ implies that, for any $k \in \{1,..., n\}$, $|\lambda_k^{(i)}(\x) - \lambda_k^{(i)}(\x^*)| \leq \bar{L}\|\x - \x^*\|$, which in turn implies $\lambda_k^{(i)}(\x) \geq \lambda_k^{(i)}(\x^*) - \bar{L}\|\x - \x^*\|$ and $\lambda_k^{(i)}(\x) \leq \lambda_k^{(i)}(\x^*) + \bar{L}\|\x - \x^*\|$. It follows that 
\begin{equation*}
    \begin{aligned}
        \log{\bar{a}} &\leq \limsup_{t}\frac{1}{t}\sum_{k = 1}^{t}\log{(1 - \frac{\bar{\lambda}_n^{o} - \bar{L}\|\x^{k_t} - \x^*\|}{\bar{\rho}_k^{o} + \bar{L}\|\x^{k_t} - \x^*\|})}\\&\stackrel{(1)}{=} \limsup_{t}\frac{1}{t}\sum_{k = 1}^{t}\log{(1 - \frac{\bar{\lambda}_n^{o} }{\bar{\rho}_k^{o} + \bar{L}\|\x^{k_t} - \x^*\|})}\\& = \limsup_{t}\frac{1}{t}\sum_{k = 1}^{t}\log{(\frac{\bar{\rho}_k^{o} - \bar{\lambda}_n^{o} + \bar{L}\|\x^{k_t} - \x^*\|}{\bar{\rho}_k^{o} + \bar{L}\|\x^{k_t} - \x^*\|})}\\&\leq  \limsup_{t}\frac{1}{t}\sum_{k = 1}^{t}\log{(1 - \frac{ \bar{\lambda}_n^{o}}{{\bar{\rho}_k^{o}}} + \frac{\bar{L}\|\x^{k_t} - \x^*\|}{\bar{\rho}_k^{o}})}\\&\stackrel{(2)}{=} \limsup_{t}\frac{1}{t}\sum_{k = 1}^{t}\log{(1 - \frac{ \bar{\lambda}_n^{o}}{{\bar{\rho}_k^{o}}})}
    \end{aligned}
\end{equation*}
where equalities (1) and (2) follow from calculations equivalent to the ones used to obtain (\ref{eq:logIdentity}).\\ 3) Starting from 2), we can apply calculations analogous to the ones used in equation (\ref{eq:periodicObtain}) of Lemma \ref{lemma:LyapLSs}.

\section*{Proof of Theorem \ref{th:suplin}}
We show that the Lyapunov exponent is $a_* = 0$. From Lemma \ref{Th:stepSizeConvex}, there exists a $\bar{t}$ such that $\eta_t = 1$ is chosen by the backtracking line search for any $t \geq \bar{t}$. Local linear convergence proven in Theorem \ref{Th:expConvergence} implies that there exists a $t'$ such that, for all $t \geq t'$, $ \|\boldsymbol{\theta}^{t+1} - \boldsymbol{\theta}^*\| \leq \bar{c}_t\|\boldsymbol{\theta}^t - \boldsymbol{\theta}^*\|$, with $\bar{c}_t < 1$. In particular, we have, from (\ref{eq:barc})
\begin{equation*}\label{eq:cbarAgain}
\bar{c}_t \leq 1-\frac{\bar{\lambda}_{n,t}}{\bar{\rho}_t} + \frac{L}{\bar{\rho}_t}\|\boldsymbol{\theta}^{k_t} - \boldsymbol{\theta}^*\| + \frac{3L}{2\bar{\rho}_t}\|\boldsymbol{\theta}^t - \boldsymbol{\theta}^*\|.    
\end{equation*}
Linear convergence implies that, for some constant $C > 0$, we can write $\|\boldsymbol{\theta}^{t} - \boldsymbol{\theta}^*\| \leq Ca^{t}$ for some $a \in (0,1)$. Furthermore, given that $k_t = t - \tau$ with $\tau$ bounded, we have $\|\x^{k_t} - \x^*\| = \|\x^{t-\tau} - \x^*\| \leq C'a^{t}$ for some bounded $C'$. 

It is easy to see that, given that the algorithm convergence is at least linear with some Lyapunov exponent $a_*$, $\bar{a}$ defined as  $\bar{a} := \limsup_{t}{(\prod_{k = 1}^{t}{\bar{c}_k})^{1/t}}$ is such that $\bar{a} \geq a_*$. For $k < t'$, $\bar{c}_k$ is some bounded value that could be greater than $1$. 

To prove the Theorem we use the fact that, for $q_t^{(i)} = n'$, $\hat{\rho}_t^{(i)} = \hat{\lambda}_{n, t}^{(i)}$ for all $i$. Let $t = Rn' + T'$ for some $T' < n'$ and $R \in \mathbb{N}$. Given the conditions required by the theorem, we see that $q_{kn'}^{(i)} = n'$ for $k = 1,2,...,R$. When $t = kn' \geq \bar{t}$, $\bar{c}_t$ is as in (\ref{eq:cbarAgain}), and we have $q_t^{(i)} = n'$ and $\hat{\rho}_{kn'}^{(i)} = \hat{\lambda}_{n, kn'}^{(i)}$, so $\bar{\rho}_{kn'} = \bar{\lambda}_{n,kn'}$. Consequently, $1-\frac{\bar{\lambda}_{n, kn'}}{\bar{\rho}_{kn'}} = 0$ and
\begin{equation*}
\bar{c}_{kn'} = \frac{L}{\bar{\rho}_{kn'}}\|\boldsymbol{\theta}^{kn' - n'} - \boldsymbol{\theta}^*\| + \frac{3L}{2\bar{\rho}_{kn'}}\|\boldsymbol{\theta}^{kn'} - \boldsymbol{\theta}^*\| \leq Ba^{kn'}    
\end{equation*}
for some bounded $B$.
Taking the logarithm of $\bar{a}$, we can then write, letting $l$ be the positive integers such that $l \geq k'$, with $k'$ a sufficiently big integer in order to have $k'n' \geq \bar{t}$
\begin{equation*}
\begin{aligned}
    \log{\bar{a}} &= \limsup_{t}{\log{(\prod_{k = 1}^{t}{\bar{c}_k})^{1/t}}} = \limsup_{t}{\frac{1}{t}}\sum_{k = 1}^{t}\log{\bar{c}_k}\\
    &= \limsup_{R}\frac{1}{Rn' + T'}(\sum_{\substack{k = 1\\ k \neq ln'}}^{Rn' + T'}{\log{\bar{c}_k}} + \sum_{k = k'}^{R}{\log{Ba^{kn'}}}),
\end{aligned}
\end{equation*}
The first term between parentheses is bounded in the following way: $\sum_{\substack{k = 1\\ k \neq ln'}}^{Rn' + T'}{\log{\bar{c}_k}} \leq C(Rn' + T')$, for some constant $C$. The second term between parentheses can be written as 
\begin{equation*}
\begin{aligned}
    \sum_{k = k'}^{R}\log{Ba^{kn'}} &= (R-k'+1)\log{B} + \sum_{k = 1}^{R}\log{a^{kn'}} - \sum_{k = 1}^{k'}\log{a^{kn'}}\\&\leq R\log{B} + (\frac{n'R^2}{2}- {n'{(k'+1)}^2})\log{a}.
\end{aligned}
\end{equation*}
The previous expression thus becomes:
\begin{equation*}
\begin{aligned}
    \log{\bar{a}} &\leq \limsup_{R}C + \frac{R\log{B} + ({n'R^2}{/2}- {n'{(k'+1)}^2})\log{a}}{Rn' + T'}\\& = C + \frac{\log{B}}{n'} + \limsup_{R}\frac{R}{2}\log{a} = -\infty
\end{aligned}
\end{equation*}
so $0 \leq a_* \leq \bar{a} = 0 \implies a_* = 0$.


\newpage
